# Supplementary material for: SmoothGNN: Smoothing-aware GNN for Unsupervised Node Anomaly Detection
Source: arXiv:2405.17525 source file (2024-10-17)
Supplement: Supplementary file 1 [file dis-appendix1.tex]

\begin{figure}[t!]
\centering
%\vspace{-4mm}
  \begin{small}
    \begin{tabular}{cc}
        \multicolumn{2}{c}{\includegraphics[height=3mm]{figures/distance/legend.eps}}  \\[-2mm]
        %\hspace{-10mm}
        \includegraphics[height=28mm]{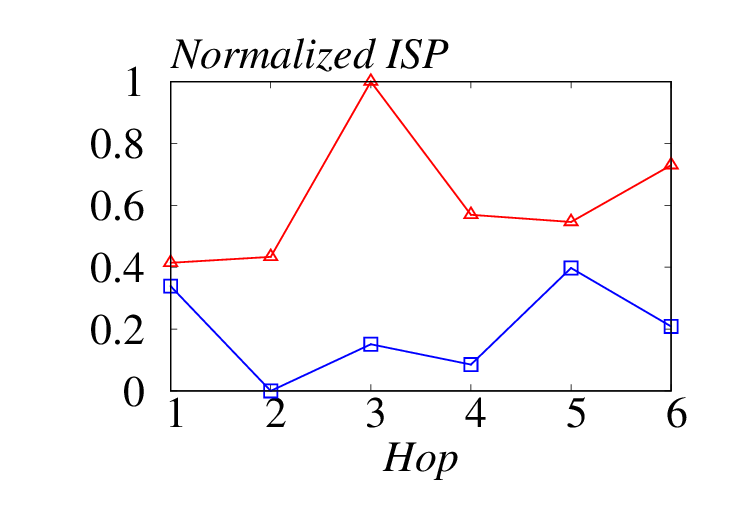} &
        %\hspace{-10mm}
        \includegraphics[height=28mm]{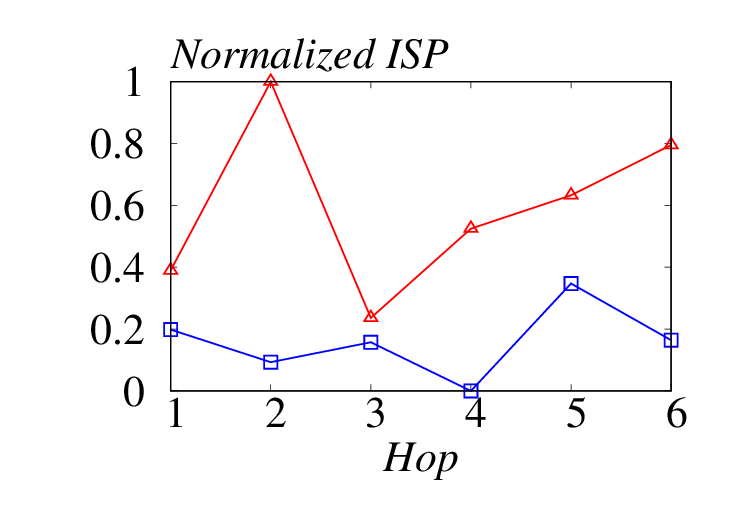} \\ [-3mm]
        %\hspace{-1mm}
        (a) Reddit & (b) Tolokers \\ [-2mm]
    \end{tabular}
    \caption{Normalized Distance from converged status on different datasets.}
    \label{fig:dis-appendix1}
    \vspace{-2mm}
  \end{small}
\end{figure}
